# Supplementary material for: Machine Learning Approaches to Automated Mechanism Design for Public Project Problem
Source: arXiv:2204.07315 source file (2022-04-15)
Supplement: Supplementary file 1 [file AppendixTemplate.tex]

\newpage
In my thesis, we study different variations of public project problems and their applications. Mechanism design for the public project is challenging. There are only a few existing mechanisms for this family of problems, and they generally do not perform well for our objectives. We find that the performance of the mechanism for these problems is greatly impacted by the scale of the number of agents. Normally, for a small number of agents, we can design a deep neural network structure or genetic algorithms to solve them. Then we can extend those mechanisms to a large number of agents. We compare our results to the theoretical upper bound and existing mechanisms. The experiments show that our mechanisms are better than previous mechanisms or very close to the theoretical upper bound.

\textbf{Firstly}, in Chapter \ref{Mechanism Design for Public Projects via Neural Networks}, we study the public project that is indivisible and binary (e.g., a bridge). Indivisible means that an agent either consumes the entire project alone or is completely excluded. Binary means that the decision of this project is to build or not to build. 
The existing methods (e.g., serial cost-sharing mechanism\cite{Moulin1994:Serial}) are not optimal in general. We prove that the serial cost-sharing mechanism is optimal in some scenarios. For other scenarios, we find the cost-sharing mechanism is far from optimal. For these scenarios, we improve existing mechanisms and design better-performing mechanisms via neural networks. We propose three neural network training techniques, and the experiments show the techniques help the mechanisms get better results than previous methods. 
%We study mechanism design for non-excludable and excludable binary public project problems. 



% \begin{itemize}
% \item For the excludable public project model,  if one agent uses it, the other agents cannot use it. We identify a sufficient condition on the prior distribution for the conservative equal costs mechanism to be the optimal strategy-proof and individually rational mechanism. 

% \item For the non-excludable public project model, if one agent uses it, the other agents can also use it. We involve three technical innovations that can be applied to mechanism design in general.  
% \begin{enumerate}
% \item We interpret the mechanisms as price-oriented rationing-free (PORF) mechanisms, which enables us to move the mechanism's complex (\emph{e.g.}, iterative)   decision making off the neural network, to a separate simulation process.  
% \item We feed the prior distribution's analytical form into the cost function to provide high-quality gradients for efficient training. 
% \item We use supervision to manual mechanisms as a systematic way for initialization. It is also effective for fixing constraint violations for heuristic-based mechanisms that are infeasible. 
% \end{enumerate}

% \end{itemize}



\textbf{Secondly}, in Chapter \ref{Public Project with Minimum Expected Release Delay}, we study the divisible public project, which means the agent can be allocated part of the project. 

In a classic excludable and non-binary public project model, we study a setting where the mechanism can set different project release times for different agents, which means, for a certain agent, he or she use the project earlier if paying higher. There are two objectives for this problem: to minimize the expected maximum release delay and to minimize the expected total release delay. The existing mechanism does not yield good results and the result is influenced by the scale of agents. For automated mechanism design, we can first find some regularities from a small number of agents and then apply them to a large number of agents. 
For a small number of agents, we propose the sequential unanimous mechanisms by extending the existing mechanisms. We use evolutionary computation to optimize the sequential unanimous mechanisms. The experiments show our mechanisms are better than the existing mechanisms. Then we manually apply these mechanisms as single deadline mechanisms into a large number of scales and theoretically prove the mechanisms are optimal for a large number of agents. We show that the optimal single deadline mechanism is asymptotically optimal for both objectives, regardless of the prior distributions.\\

\textbf{Moreover}, in Chapter \ref{Redistribution in Public Project Problems via Neural Networks}, we focus on the VCG and VCG redistribution (which is based on VCG) mechanisms for the classic public project problem. We design mechanisms via neural networks with two welfare-maximizing objectives: optimal in the worst case and optimal in expectation. The neural networks are not restricted by the limitations of classical methods and thus can easily deal with different prior input distributions. 
For the worst-case objective, we conduct a generative adversarial network (GAN) to minimize the worst-case performance of redistribution mechanisms in public project problems. The experiments show our approaches are better than all the existing approaches. 
We use multi-layer perceptions (MLP) to find the optimal-in-expectation for VCG redistribution mechanism in public project problems. The experiments show our mechanisms are very close to the theoretical upper bound.

\textbf{At last}, in Chapter \ref{Revenue-Maximizing Markets for Zero-Day Exploits}, we use aforementioned methods to design numerical solution techniques on zero-day exploit market. In zero-day exploit market, a group of offenders and defenders compete to buy the zero-day exploit information. We study the problem of selling one zero-day exploit (as a public project) to multiple defenders and offenders. It can be regarded as a specific public project problem. For revenue maximization in zero-day exploit markets, we adopt computational feasible technical automated mechanism design approaches \cite{Guo2017:Optimizing}. One commonly used mechanism for revenue maximization in computational feasible technical automated mechanism design is Affine Maximizer Auctions (AMA). For this particular model, we find AMA mechanisms can be regarded as a simple variable function that can be visualized as a curve. We propose two numerical solution techniques, which are based on neural networks and evolutionary computation, respectively.
We use neural networks to automatically get the optimal curve for AMA mechanisms. We also use evolutionary computation based on Fourier series to optimize AMA mechanisms. The experiments show our mechanisms based on neural networks and evolutionary computation are near-optimal and better than the state of the art method, which is based on iterative linear programming (LP).
